# Supplementary material for: Stochastic Runge-Kutta Accelerates Langevin Monte Carlo and Beyond
Source: arXiv:1906.07868 source file (2020-02-01)
Supplement: Supplementary file 1 [file ito_cal.tex]

\section{Background on It\^o Calculus} \label{app:ito_cal}
In this section, we provide background on the results in It\^o calculus which 
will be used throughout our analyses and proofs. We refer the serious reader 
to~\cite{oksendal2003stochastic} for an in-depth treatment.

\paragraph{It\^o's Lemma} It\^o's Lemma (or It\^o's formula) is the backbone of 
It\^o stochastic calculus. On a high-level, the lemma can be understood 
as the stochastic calculus counterpart of the chain rule.

\begin{theo}[It\^o's Lemma]
Let $\{X_t\}_{t\ge0}$ be an $d$-dimensional It\^o process adapted to the natural filtration 
$\{\F_t\}_{t\ge0}$ of the $d$-dimensional Brownian motion $\{B_t\}_{t\ge0}$. 
If $f: \R^d \to \R$ is twice differentiable, then $Y_t = f(X_t)$ is also 
an It\^o process, and 
\eqn{
    \dY_t = 
        \abracks{ \nabla f(X_t), \dX_t } + \frac{1}{2} \nabla^2 f(X_t) [\dX_t, \, \dX_t], \numberthis
}
where $\dX_t^{(i)} \dX_t^{(j)}$ is computed using the rules
\eqn{
    &\dt \dt = \dt \dB_t^{(i)} = \dt \dB_t^{(j)} = 0,\quad 
    \dB_t^{(i)} \dB_t^{(j)} = 
        \begin{cases}
        0   \,\,\,\quad i \ne j \\
        \dt \quad i = j
        \end{cases}. \numberthis
}
\end{theo}

\paragraph{It\^o Isometry} It\^o isometry provides a way to compute the variance of 
It\^o integrals of adapted processes. We first provide a theorem for single-dimensional
integrals, and later note that the result can be extended to vector-valued integrals.

\begin{theo}[It\^o Isometry]
Let $\{X_t\}_{t\ge0}$ be a single-dimensional stochastic process adapted to the natural
filtration $\{\F_t\}_{t\ge0}$ of the single-dimensional Brownian motion $\{B_t\}_{t\ge0}$. 
Then,
\eqn{
    \E \biggl[
        \Bigl( \int_0^t X_s \dB_s \Bigr)^2
    \biggr]
    =
    \Exp{ \int_0^t X_s^2 \ds }. \numberthis
}
\end{theo}

The theorem also holds for vector-valued integrals, i.e.
\eqn{
    \E \biggl[
        \Bigl( \int_0^t X_s \dB_s \Bigr)^2
    \biggr]
    =
    \Exp{
        \int_0^t \normf{X_s}^2 \ds
    }. \numberthis
}
